# Supplementary material for: Variable Independence in Linear Real Arithmetic
Source: arXiv:2307.09499 source file (2023-07-18)
Supplement: Supplementary file 1 [file appendix_prepend.tex]

% prepend "Appendix" to all titles of appendices
\makeatletter
\newcommand\appendix@section[1]{%
	\refstepcounter{section}%
	\orig@section*{Appendix \@Alph\c@section: #1}%
	\addcontentsline{toc}{section}{Appendix \@Alph\c@section: #1}%
}
\let\orig@section\section
\g@addto@macro\appendix{\let\section\appendix@section}
\makeatother
